# Supplementary material for: Full-Body Awareness from Partial Observations
Source: arXiv:2008.06046 source file (2020-08-13)
Supplement: Supplementary file 1 [file ct.tex]

\clearpage
\subsection{Random Results on Cross-Task} \label{sec:ct}
\begin{multicols}{2}
\begin{tabular}{ccc}
\includegraphics[width = 1.9in]{supplemental/IV_imgs/ire_0021_00002033.jpg} &
\includegraphics[width = 1.9in]{supplemental/IV_imgs/pot_0014_00002499.jpg} &
\includegraphics[width = 1.9in]{supplemental/IV_imgs/pot_0028_00009018.jpg} \\
\includegraphics[width = 1.9in]{supplemental/IV_imgs/ire_0009_00019067.jpg} &
\includegraphics[width = 1.9in]{supplemental/IV_imgs/cpr_0026_00001728.jpg} &
\includegraphics[width = 1.9in]{supplemental/IV_imgs/ire_0029_00009321.jpg} \\
\includegraphics[width = 1.9in]{supplemental/IV_imgs/cpr_0009_00002382.jpg} &
\includegraphics[width = 1.9in]{supplemental/IV_imgs/fee_0015_00008326.jpg} &
\includegraphics[width = 1.9in]{supplemental/IV_imgs/ire_0011_00003163.jpg} \\
\end{tabular}
\end{multicols}
\vspace{2em}
