# Supplementary material for: Full-Body Awareness from Partial Observations
Source: arXiv:2008.06046 source file (2020-08-13)
Supplement: Supplementary file 3 [file vlog.tex]

\subsection{Random Results on VLOG} \label{sec:sec_vlog}

\begin{figure}[h!]
	\centering
			{\includegraphics[width=\textwidth]{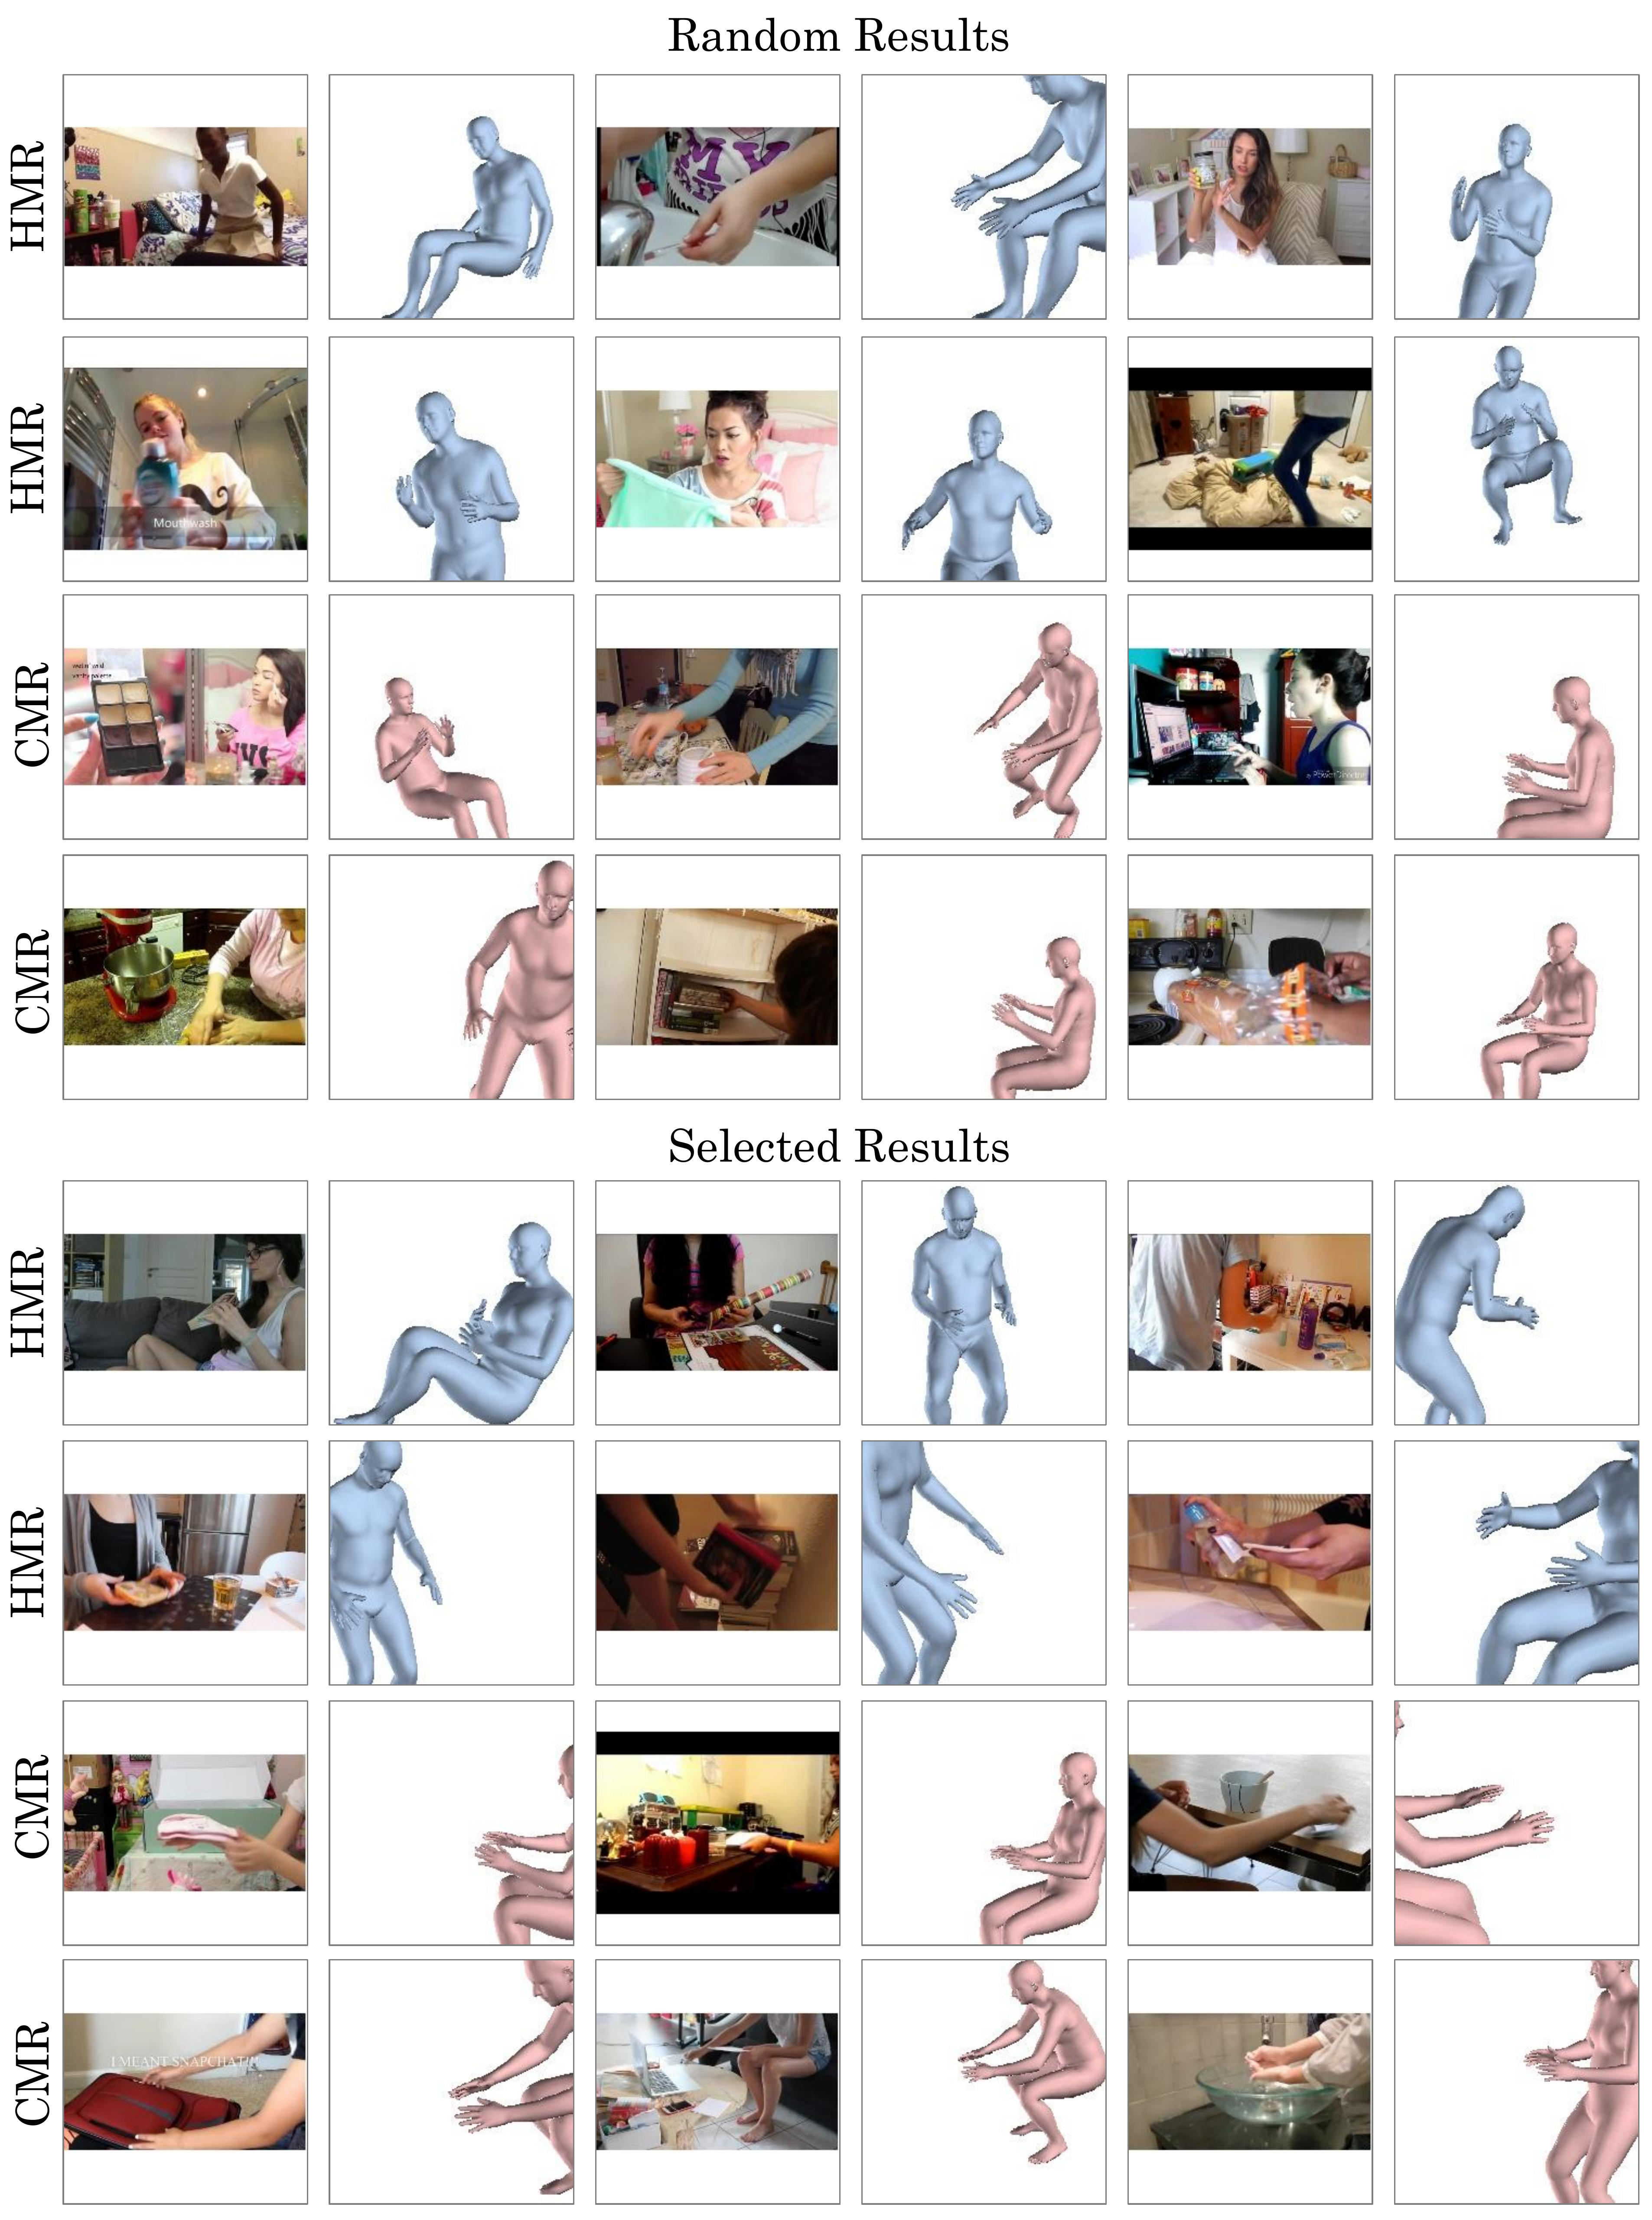}}
\end{figure}
