# Supplementary material for: Full-Body Awareness from Partial Observations
Source: arXiv:2008.06046 source file (2020-08-13)
Supplement: Supplementary file 4 [file yc.tex]

\subsection{Random Results on YouCookII} \label{sec:yc}
\begin{multicols}{2}
\begin{tabular}{ccc}
\includegraphics[width = 1.9in]{supplemental/yc_imgs/4y7y5BCY_00006340.jpg} &
\includegraphics[width = 1.9in]{supplemental/yc_imgs/kTiH5juI_00006330.jpg} &
\includegraphics[width = 1.9in]{supplemental/yc_imgs/kN3LASfo_00002230.jpg} \\
\includegraphics[width = 1.9in]{supplemental/yc_imgs/0ANIXrLc_00001994.jpg} &
\includegraphics[width = 1.9in]{supplemental/yc_imgs/3FfR5gOY_00010556.jpg} &
\includegraphics[width = 1.9in]{supplemental/yc_imgs/0eDJ4lyY_00005774.jpg} \\
\includegraphics[width = 1.9in]{supplemental/yc_imgs/wQJQKR5Y_00003957.jpg} &
\includegraphics[width = 1.9in]{supplemental/yc_imgs/ri1Sg6qU_00002534.jpg} &
\includegraphics[width = 1.9in]{supplemental/yc_imgs/jentYJbg_00010222.jpg} \\
\end{tabular}
\centering
\end{multicols}
